# Supplementary material for: Hierarchically Structured Neural Bones for Reconstructing Animatable Objects from Casual Videos
Source: arXiv:2408.00351 source file (2024-08-01)
Supplement: Supplementary file 1 [file dynamic_tree.tex]

\begin{figure}[t]
    \centering
    \includegraphics[width=1\linewidth]{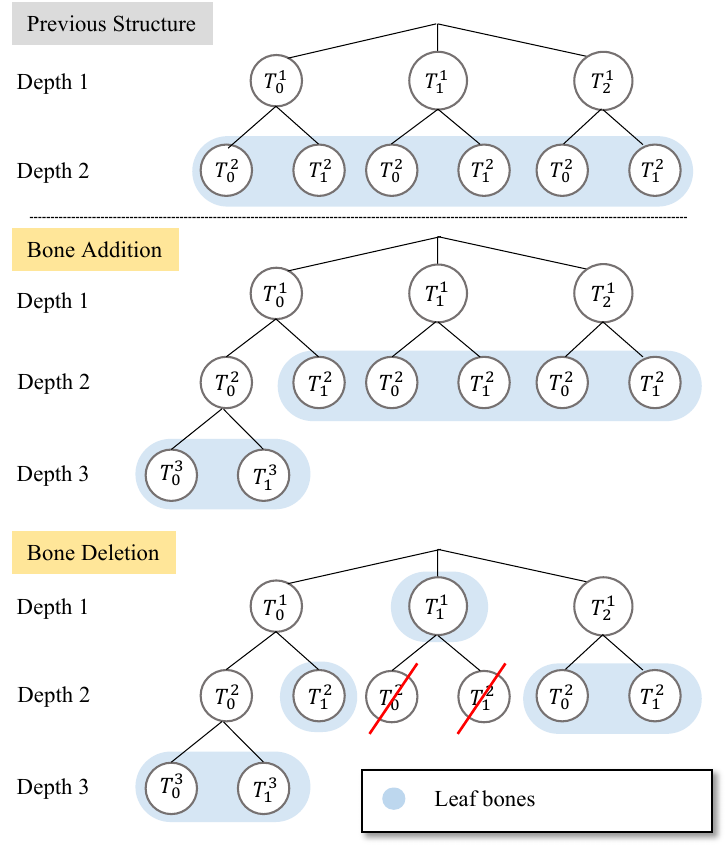}
    \caption{Dynamic addition and deletion of neural bones.}
    \label{fig:dynamic_tree}
\end{figure}
